# Supplementary material for: Excited state, non-adiabatic dynamics of large photoswitchable molecules using a chemically transferable machine learning potential
Source: arXiv:2108.04879 source file (2022-03-16)
Supplement: Supplementary file 1 [file sm_preamble.tex]

\usepackage{amsthm}
\usepackage{mathtools}
\usepackage{physics}
\usepackage{xcolor}
\usepackage{graphicx}
\usepackage[left=23mm,right=13mm,top=35mm,columnsep=15pt]{geometry} 
\usepackage{adjustbox}
\usepackage{placeins}
\usepackage[T1]{fontenc}
\usepackage{lipsum}
\usepackage{csquotes}
\usepackage{scrextend}
\usepackage{booktabs}
\usepackage{multibib}
\usepackage{multirow} 
\usepackage{xltabular}
\usepackage{epstopdf}
\usepackage{xr} % For references to external documents


\setlength {\marginparwidth }{2cm} 
\makeatletter
\newcommand\footnoteref[1]{\protected@xdef\@thefnmark{\ref{#1}}\@footnotemark}
\makeatother


\raggedbottom % to avoid extra lines - these are added to make every page end at the very bottom


% For references to external documents

\makeatletter
\newcommand*{\addFileDependency}[1]{% argument=file name and extension
  \typeout{(#1)}
  \@addtofilelist{#1}
  \IfFileExists{#1}{}{\typeout{No file #1.}}
}
\makeatother

\newcommand*{\myexternaldocument}[2][]{%
    \externaldocument[#1]{#2}%
    \addFileDependency{#2.tex}%
    \addFileDependency{#2.aux}%
}

\myexternaldocument{main}
